# Supplementary material for: Finding Safe Zones of policies Markov Decision Processes
Source: arXiv:2202.11593 source file (2023-10-09)
Supplement: Supplementary file 1 [file sup-6_hardness.tex]

% commented out- now inside appendix A

% \theoremReductionCorrectness*
% \begin{proof}
% $(\Longrightarrow)$ If there is a clique of size $k_c$, then we can take the corresponding $k$ states. The probability to remain in this subset is at least $\left(\frac{k-1}{d}\right)^2$ (remember that $H=2$). Thus, an exact solver for $\newprob$ must return YES.

% $(\Longleftarrow)$ Suppose there is no clique of size $k$. Assume by contradiction that the reduction (algorithm) returns YES. Let $s_0$ be a vertex which was the starting state from the running instance which the YES came from and let $\hat{F}$ denote the output of \newprob. We will show that the probability to remain in any subset of size $k$ is smaller than $\left(\frac{k-1}{d}\right)^2$.

% Since there is no clique of size $k$ in $G$, we know that $\hat{F}$ is not a clique. It therefore follows that there exists at least two vertexes, $s_a,s_b\in V$ such that $(s_a,s_b)\notin E$. 

% We will now bound the probability of escape from state $s_0$ by exhaustion.
% \begin{enumerate}
%     \item If $s_0\ne s_a$, then 
%     \[
%     \Pr[escape\;from\; s_0]\geq \Pr[t=1:(s_0,s'),s'\notin \hat{F}]
%     \]
%     \[
%     +\Pr[t=1:(s_0,s),s\ne s_a]\cdot \Pr[t=2:(s,s'),s'\notin \hat{F}|t=1:(s_0,s), s\ne s_a]
%     \]
%     \[
%     +\Pr[t=1:(s_0,s_a)]\cdot \Pr[t=2:(s_a,s'),s'\notin \hat{F}|t=1:(s_0,s_a)]
%     \]
%     \[
%     =\frac{d-(k-1)}{d}+\frac{k-2}{d}\cdot \frac{d-(k-1)}{d}
%     +\frac{1}{d}\cdot \frac{d-(k-2)}{d}
%     \]
%     \[
%     = 1-\frac{k-1}{d}+\frac{k-2}{d}-\frac{(k-2)(k-1)}{d^2}+\frac{1}{d}-\frac{k-2}{d^2}=
%     \]
%     \[
%     1-\frac{k-2}{d^2}(k-1+1)=1-\frac{k(k-2)}{d^2}
%     \]
%     Hence
%     \[
%     \Pr[staying]\leq \frac{k(k-2)}{d^2} <\frac{(k-1)^2}{d^2}.
%     \]
    
%     \item If $s_0= s_a$, then 
%     \[
%     \Pr[escape\;from\; s_0]\geq \Pr[t=1:(s_0,s'),s'\notin \hat{F}]
%     \]
%     \[
%     +\Pr[t=1:(s_0,s),s\in \hat{F}]\cdot \Pr[t=2:(s,s'),s'\notin \hat{F}|t=1:(s_0,s), s\in \hat{F}]
%     \]
%     \[
%     =\frac{d-(k-2)}{d}+\frac{k-2}{d}\cdot \frac{d-(k-1)}{d}
%     \]
%     \[
%     = 1-\frac{k-2}{d}+\frac{k-2}{d}-\frac{(k-2)(k-1)}{d^2}
%     \]
%     \[
%     =1-\frac{(k-2)(k-1)}{d^2}
%     \]
%     Hence
%     \[
%     \Pr[staying]\leq \frac{(k-2)(k-1)}{d^2} <\frac{(k-1)^2}{d^2}.
%     \]
% \end{enumerate}
% \end{proof}
